# Supplementary material for: Predictive power-sharing scaling law in double-null L-mode plasmas
Source: arXiv:2406.19684 source file (2024-06-28)
Supplement: Supplementary file 1 [file 8_Appendix.tex]

\section{Appendix}\label{Appendix:1}
